# Supplementary material for: N-Representability Violations in Truncated Equation-of-Motion Coupled-Cluster Methods
Source: arXiv:2305.06457 ancillary file (2023-07-12)
Supplement: Supplementary file 1 [file tdcc_gpc_sm.pdf]

# Supporting Information for: $N$-Representability Violations in Truncated Equation-of-Motion Coupled-Cluster Methods

Stephen H. Yuwono and A. Eugene DePrince III[a)]

*Department of Chemistry and Biochemistry, Florida State University, Tallahassee, FL 32306-4390, USA*

[a)]Electronic mail: adeprince@fsu.edu

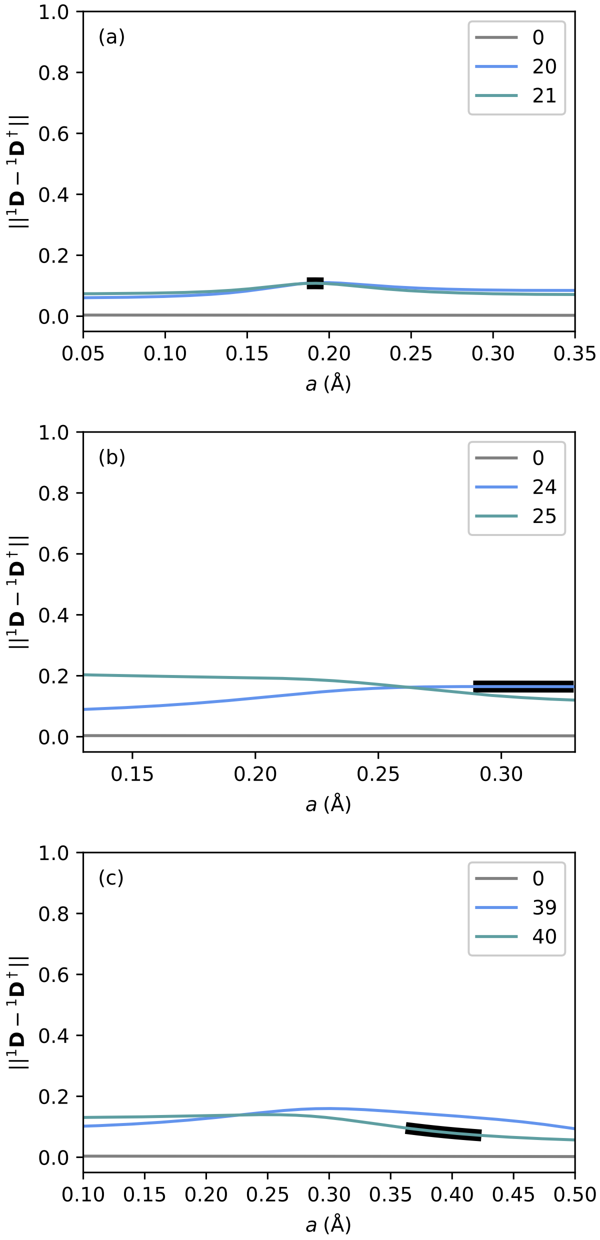


FIG. S1. Non-hermiticity metric characterizing the 1RDMs of the states reported in Fig. 2 of the main text. The ground-state non-hermiticity measure is included for comparison.

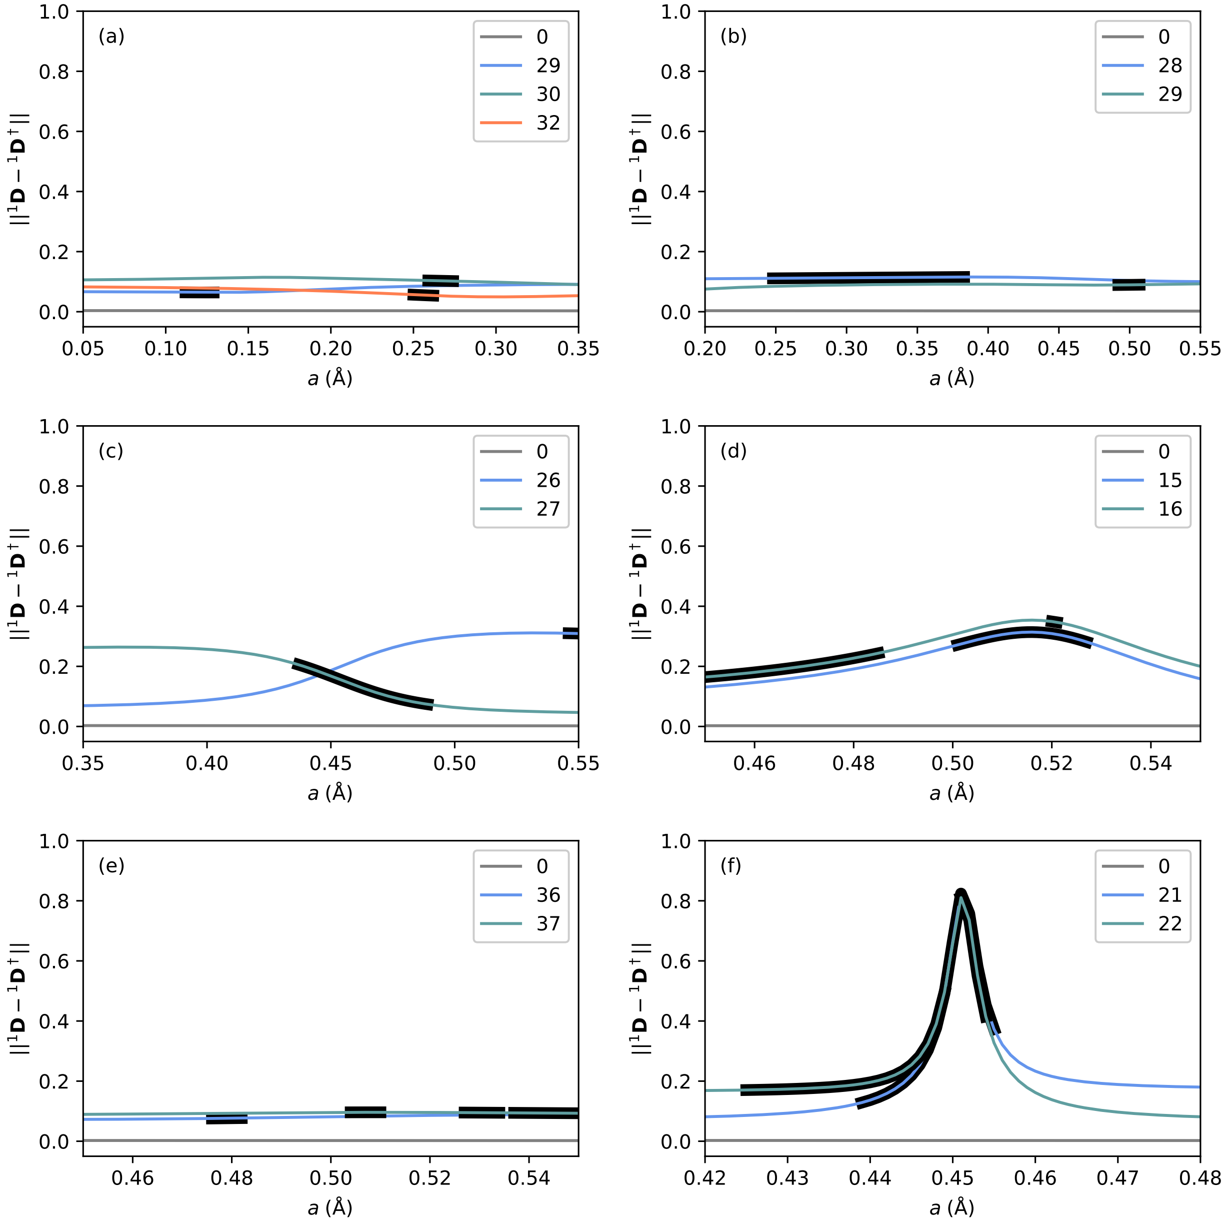


FIG. S2. Non-hermiticity metric characterizing the 1RDMs of the states reported in Fig. 3 of the main text. The ground-state non-hermiticity measure is included for comparison.

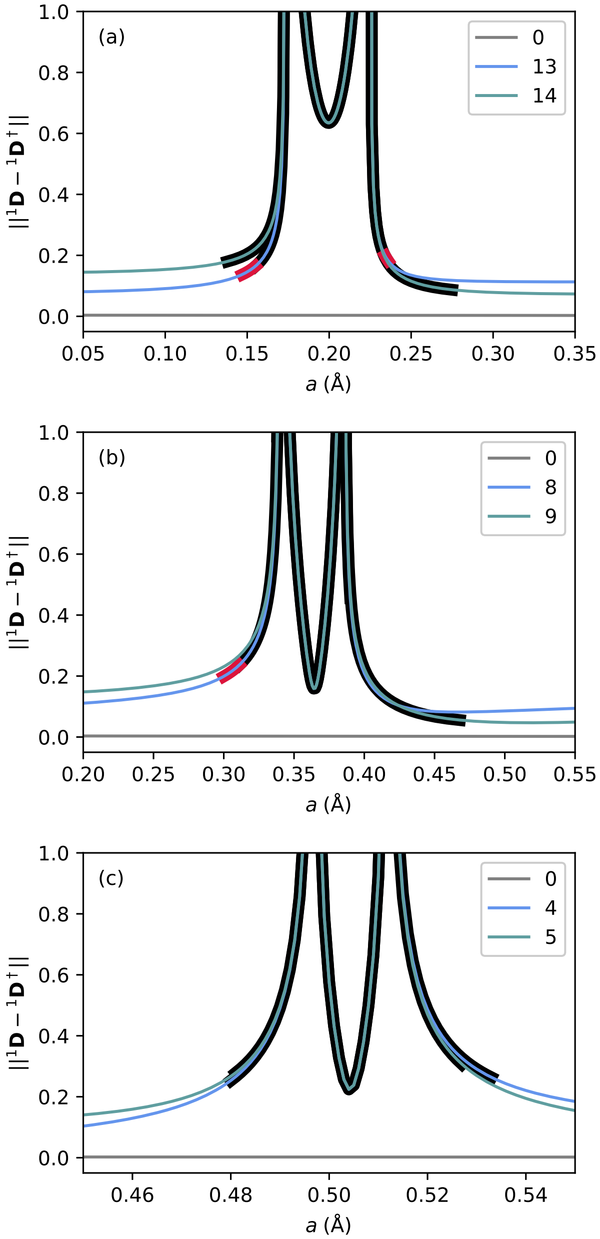


FIG. S3. Non-hermiticity metric characterizing the 1RDMs of the states reported in Fig. 4 of the main text. The ground-state non-hermiticity measure is included for comparison.
